# Supplementary material for: Blind Image Restoration via Fast Diffusion Inversion
Source: arXiv:2405.19572 source file (2024-11-05)
Supplement: Supplementary file 1 [file suppl_old.tex]

%\documentclass{article}
\documentclass[runningheads]{llncs}

% ---------------------------------------------------------------
% Include basic ECCV package
 
% TODO REVIEW: Insert your submission number below by replacing '*****'
% TODO FINAL: Comment out the following line for the camera-ready version
\usepackage[review,year=2024,ID=10477]{eccv}
% TODO FINAL: Un-comment the following line for the camera-ready version
%\usepackage{eccv}

% OPTIONAL: Un-comment the following line for a version which is easier to read
% on small portrait-orientation screens (e.g., mobile phones, or beside other windows)
%\usepackage[mobile]{eccv}


% ---------------------------------------------------------------
% Other packages

% Commonly used abbreviations (\eg, \ie, \etc, \cf, \etal, etc.)
\usepackage{eccvabbrv}

% Include other packages here, before hyperref.
\usepackage{graphicx}
\usepackage{booktabs}
\usepackage{algorithm}
\usepackage{algorithmic}
\usepackage{tabularx}
\usepackage{multirow}
\usepackage{amssymb}
\usepackage{amsmath} % for the equation* environment
\usepackage{subfigure}
% The "axessiblity" package can be found at: https://ctan.org/pkg/axessibility?lang=en
\usepackage[accsupp]{axessibility}  % Improves PDF readability for those with disabilities.


% ---------------------------------------------------------------
% Hyperref package

% It is strongly recommended to use hyperref, especially for the review version.
% Please disable hyperref *only* if you encounter grave issues.
% hyperref with option pagebackref eases the reviewers' job, but should be disabled for the final version.
%
% If you comment hyperref and then uncomment it, you should delete
% main.aux before re-running LaTeX.
% (Or just hit 'q' on the first LaTeX run, let it finish, and you
%  should be clear).

% TODO FINAL: Comment out the following line for the camera-ready version
\usepackage[pagebackref,breaklinks,colorlinks,citecolor=eccvblue]{hyperref}
% TODO FINAL: Un-comment the following line for the camera-ready version
%\usepackage{hyperref}

% Support for ORCID icon
\usepackage{orcidlink}


% %\newcommand{\R}{\mathbb{R}}
% \newcommand{\I}{\mathbf{I}}
% %\newcommand{\E}{\mathbf{E}}
% \newcommand{\N}{\mathcal{N}}
% \newcommand{\D}{\mathcal{D}}

% % \newcommand{\etal}{\textit{et al}.}
% % \newcommand{\ie}{\textit{i}.\textit{e}.}
% % \newcommand{\eg}{\textit{e}.\textit{g}.}
% % \newcommand{\cf}{\textit{c}.\textit{f}.}

\newcommand{\methodName}{SHRED\xspace}


%\title{Zero-shot Image Restoration via Diffusion Inversion}



%\newcommand{\methodNameExpanded}{...}


\title{Zero-shot Image Restoration through Diffusion Inversion}
\title{Zero-shot Image Restoration via Diffusion Inversion}

% The \author macro works with any number of authors. There are two commands
% used to separate the names and addresses of multiple authors: \And and \AND.
%
% Using \And between authors leaves it to LaTeX to determine where to break the
% lines. Using \AND forces a line break at that point. So, if LaTeX puts 3 of 4
% authors names on the first line, and the last on the second line, try using
% \AND instead of \And before the third author name.


\author{%
  David S.~Hippocampus\thanks{Use footnote for providing further information
    about author (webpage, alternative address)---\emph{not} for acknowledging
    funding agencies.} \\
  Department of Computer Science\\
  Cranberry-Lemon University\\
  Pittsburgh, PA 15213 \\
  \texttt{hippo@cs.cranberry-lemon.edu} \\
  % examples of more authors
  % \And
  % Coauthor \\
  % Affiliation \\
  % Address \\
  % \texttt{email} \\
  % \AND
  % Coauthor \\
  % Affiliation \\
  % Address \\
  % \texttt{email} \\
  % \And
  % Coauthor \\
  % Affiliation \\
  % Address \\
  % \texttt{email} \\
  % \And
  % Coauthor \\
  % Affiliation \\
  % Address \\
  % \texttt{email} \\
}


\begin{document}

\maketitle
\section{Implementation Details}

In the next sections, we show the implementation details in terms of degradation operators and training hyper-parameters for every degradation task. We also provide runtime comparisons between the different methods.

% \usepackage{booktabs}



\subsection{Super-Resolution}
For superresolution, we use $\times 4$, $\times 8$, and $\times 16$ uniform downsampling factors for ImageNet and $\times 8$, $\times 16$, and $\times 32$ uniform downsampling factors for CelebA. During training, we use Adam as our optimizer with a learning rate of $0.01$ and $300$ iterations. We also add comparisons with both OID~\cite{chen2020oid} and Chen et al.~\cite{chen2020enhanced} . Additional visual results are depicted in \cref{fig:supres1}, \cref{fig:supres2} and \cref{fig:supres3}. While other methods tend to generate over-smoothed images especially at higher downsampling factors, our method (SHRED) outputs sharper and more realistic images. For instance, SHRED is able to generate detailed grass and hair textures in \cref{fig:supres1} and \cref{fig:supres2} especially at $\times 16$ upscaling where other methods fail.

\subsection{Blind Deconvolution}

For Blind Deconvolution, we apply a random anisotropic Gaussian kernel of size 41x41. During training, we use Adam as our optimizer with a learning rate of $0.001$ and $300$ iterations. Visual results are shown in  \cref{fig:deblur1} and \cref{fig:deblur2}. Despite the heavy blur, SHRED is able to better deblur the main object present in the considered image compared to other methods.


\subsection{Compressed Sensing (CS)}
For Compressed Sensing, 
% we apply a subsampling of ratios $1\%$ and $5\%$ in the pixels space. 
we randomly subsample $1\%$ and $5\%$ of the total available pixels.
During training, we use Adam as our optimizer with a learning rate of $0.01$ and $400$ iterations. More visual results are depicted in \cref{fig:cs1} and \cref{fig:cs2}. SHRED performs better than the other methods at preserving the identity of the original image especially at the higher subsampling rates. Indeed, we see in the second and forth rows of \cref{fig:cs1} that other method hallucinate new faces instead of reconstructing the correct one.

\subsection{Inpainting}
For Inpainting, we apply a square mask for CelebA and a text mask for ImageNet.  During training, we use Adam as our optimizer with a learning rate of $0.01$ and $400$ iterations. We show additional results with different masks in \cref{fig:inpainting} and \cref{fig:inpainting2}.


\subsection{Runtime}
In \cref{tab:runtime}, we report the runtime per image of the different compared methods. Despite being an iterative method, SHRED has a reasonable runtime making it a practical zero-shot method. In fact, for both super-resolution and blind deblurring, SHRED needs around 4 minutes per image and around 5 minutes per image for both inpainting and compressed sensing. 


\begin{table}[t]
\centering
\small
\caption{Runtime (in seconds) comparison of different methods on CelebA per image. All experiments are conducted on a Geforce GTX 1080 Ti.}
\label{tab:runtime}
\begin{tabular}{@{}lcccc@{}}
\toprule
Method     & Inpainting & Super-Resolution & Blind Deconvolution & Compressed Sensing \\ \midrule
DIP~\cite{ulyanov2018deep}        &       520     &      520           &    -                 &       -              \\
SelfDeblur~\cite{ren2020neural} &        -    &      -          &   173                  &       -              \\
RePaint~\cite{lugmayr2022repaint}    &      482      &       -         &   -                  &              482       \\
DDRM~\cite{kawar2022denoising}       &         13   &          -      &  -                   &      13               \\
DDNM~\cite{wang2022zero}       &        12    &         12       &      -               &    12                 \\
SHRED      &      328      &           244     &         244            &      328               \\ \bottomrule
\end{tabular}
\end{table}

\begin{figure}[t]

    \setkeys{Gin}{width=0.16\linewidth}
    \captionsetup[subfigure]{skip=0.5ex,
                             belowskip=0.5ex,
                             labelformat=simple}
    \renewcommand\thesubfigure{}
    \setlength\tabcolsep{1.pt}
    %\setlength\baselineskip{0.5pt}
    \small
    \centering
  \begin{tabular}{cccccc}

  \textit{Masked} & \textit{Repaint} & \textit{ DDRM } &\textit{DDNM} & \textit{\methodName} & \textit{ GT } \\
%\rotatebox[origin=l]{90}{\textit{Masked}} & 
{\includegraphics{images/supple/celeba/inpainting/masked_258.png}}& {\includegraphics{images/supple/celeba/inpainting/repaint_258_square.png}}& {\includegraphics{images/supple/celeba/inpainting/ddrm_258_square.png}} & {\includegraphics{images/supple/celeba/inpainting/ddnm_258_square.png}}& {\includegraphics{images/supple/celeba/inpainting/ours_258.png}}& {\includegraphics{images/supple/celeba/inpainting/00258.png}} \\
 % & \textit{18.72} & \textit{31.30} & \textit{31.38} & \textit{31.25} & \textbf{\textit{31.46}} \\
%\vspace{-1cm}

{\includegraphics{images/supple/celeba/inpainting/masked_258_mask.png}}& {\includegraphics{images/supple/celeba/inpainting/repaint_258_mask.png}}& {\includegraphics{images/supple/celeba/inpainting/ddrm_258_mask.png}}&{\includegraphics{images/supple/celeba/inpainting/ddnm_258_mask.png}}& {\includegraphics{images/supple/celeba/inpainting/ours_258_mask.png}}& {\includegraphics{images/supple/celeba/inpainting/00258.png}}  \\

{\includegraphics{images/supple/celeba/inpainting/masked_258_lorem.png}}& {\includegraphics{images/supple/celeba/inpainting/repaint_258_lorem.png}}& {\includegraphics{images/supple/celeba/inpainting/ddrm_258_lorem.png}}&{\includegraphics{images/supple/celeba/inpainting/ddnm_258_lorem.png}}& {\includegraphics{images/supple/celeba/inpainting/ours_258_lorem.png}}& {\includegraphics{images/supple/celeba/inpainting/00258.png}}  \\


%\rotatebox[origin=l]{90}{\textit{DDRM}} & 
{\includegraphics{images/supple/celeba/inpainting/masked_416_square.png}}&{\includegraphics{images/supple/celeba/inpainting/repaint_416_square.png}}& {\includegraphics{images/supple/celeba/inpainting/ddrm_416_square.png}}&{\includegraphics{images/supple/celeba/inpainting/ddnm_416_square.png}}& {\includegraphics{images/supple/celeba/inpainting/ours_416_square.png}}& {\includegraphics{images/supple/celeba/inpainting/00416.png}}  \\
% & \textit{18.80} & \textit{24.23} & \textit{29.14} & \textit{31.14} & \textbf{\textit{31.28}} \\

%\rotatebox[origin=l]{90}{\textit{DDRM}} & 
{\includegraphics{images/supple/celeba/inpainting/masked_416_mask.png}}& {\includegraphics{images/supple/celeba/inpainting/repaint_416_mask.png}}& {\includegraphics{images/supple/celeba/inpainting/ddrm_416_mask.png}}&{\includegraphics{images/supple/celeba/inpainting/ddnm_416_mask.png}}& {\includegraphics{images/supple/celeba/inpainting/ours_416_mask.png}}& {\includegraphics{images/supple/celeba/inpainting/00416.png}}  \\


{\includegraphics{images/supple/celeba/inpainting/masked_416_lorem.png}}& {\includegraphics{images/supple/celeba/inpainting/repaint_416_lorem.png}}& {\includegraphics{images/supple/celeba/inpainting/ddrm_416_lorem.png}}&{\includegraphics{images/supple/celeba/inpainting/ddnm_416_lorem.png}}& {\includegraphics{images/supple/celeba/inpainting/ours_416_lorem.png}}& {\includegraphics{images/supple/celeba/inpainting/00416.png}}  \\


   \end{tabular}
% \captionof{figure}{\label{fig:inpainting} Visual results of inpaintings }
\caption{Visual results of inpaintings on CelebA.}
\label{fig:inpainting} 
\end{figure}




\begin{figure}[h]

    \setkeys{Gin}{width=0.16\linewidth}
    \captionsetup[subfigure]{skip=0.5ex,
                             belowskip=0.5ex,
                             labelformat=simple}
    \renewcommand\thesubfigure{}
    \setlength\tabcolsep{1.pt}
    %\setlength\baselineskip{0.5pt}
    \small
    \centering
  \begin{tabular}{cccccc}

  \textit{Masked} & \textit{Repaint} & \textit{ DDRM } &\textit{DDNM} & \textit{\methodName} & \textit{ GT } \\
%\rotatebox[origin=l]{90}{\textit{Masked}} & 
{\includegraphics{images/supple/imagenet/inpainting/masked_28_imagenet.png}}& {\includegraphics{images/supple/imagenet/inpainting/repaint_28_square.png}}& {\includegraphics{images/supple/imagenet/inpainting/ddrm_28_square.png}} & {\includegraphics{images/supple/imagenet/inpainting/ddnm_303_square.png}}& {\includegraphics{images/supple/imagenet/inpainting/ours_28_square_imagenet.png}}& {\includegraphics{images/supple/imagenet/inpainting/28.png}} \\
 % & \textit{18.72} & \textit{31.30} & \textit{31.38} & \textit{31.25} & \textbf{\textit{31.46}} \\
%\vspace{-1cm}

%\rotatebox[origin=l]{90}{\textit{DDRM}} & 
{\includegraphics{images/supple/imagenet/inpainting/masked_28_lorem.png}}& {\includegraphics{images/supple/imagenet/inpainting/ddrm_28_lorem.png}}& {\includegraphics{images/supple/imagenet/inpainting/ddrm_28_lorem.png}} & {\includegraphics{images/supple/imagenet/inpainting/ddnm_28_lorem.png}}& {\includegraphics{images/supple/imagenet/inpainting/ddrm_28_lorem.png}}& {\includegraphics{images/supple/imagenet/inpainting/28.png}} \\
% & \textit{18.80} & \textit{24.23} & \textit{29.14} & \textit{31.14} & \textbf{\textit{31.28}} \\


%\rotatebox[origin=l]{90}{\textit{DDRM}} & 
{\includegraphics{images/supple/imagenet/inpainting/masked_303_imagenet.png}}& {\includegraphics{images/supple/imagenet/inpainting/repaint_303_square.png}}& {\includegraphics{images/supple/imagenet/inpainting/ddrm_303_square.png}} & {\includegraphics{images/supple/imagenet/inpainting/ddnm_28_square.png}}& {\includegraphics{images/supple/imagenet/inpainting/ours_303_square_imagenet.png}}& {\includegraphics{images/supple/imagenet/inpainting/303.png}} \\
 % & \textit{18.72} & \textit{31.30} & \textit{31.38} & \textit{31.25} & \textbf{\textit{31.46}} \\
%\vspace{-1cm}

%\rotatebox[origin=l]{90}{\textit{DDRM}} & 
{\includegraphics{images/supple/imagenet/inpainting/masked_303_lorem.png}}& {\includegraphics{images/supple/imagenet/inpainting/ddnm_303_lorem.png}}& {\includegraphics{images/supple/imagenet/inpainting/ddrm_303_lorem.png}} & {\includegraphics{images/supple/imagenet/inpainting/ddnm_303_lorem.png}}& {\includegraphics{images/supple/imagenet/inpainting/ddrm_303_lorem.png}}& {\includegraphics{images/supple/imagenet/inpainting/303.png}} \\


   \end{tabular}
% \captionof{figure}{\label{fig:inpainting} Visual results of inpaintings }
\caption{Visual results of inpaintings on ImageNet.}
\label{fig:inpainting2} 
\end{figure}



%%%%%%%%%% SR updated Figure %%%%%%%%%%%%%%%
\begin{figure}[t]

\setkeys{Gin}{width=0.16\linewidth}
\setlength\tabcolsep{1.pt}
    % \captionsetup[subfigure]{skip=0.5ex,
    %                          belowskip=0.5ex,
    %                          labelformat=simple}
    % \renewcommand\thesubfigure{}
    % \setlength\tabcolsep{1.pt}
    
\subfigure{
\centering
    \small
  \begin{tabular}{lccc}

  & \textit{$\times$8} & \textit{$\times$16} & \textit{ $\times$32 } \\
\rotatebox[origin=l]{90}{\qquad\textit{Bicubic}} & {\includegraphics{images/supple/celeba/sr/bicubic_x8_00274.png}}& {\includegraphics{images/supple/celeba/sr/bicubic_x16_00274.png}}& {\includegraphics{images/supple/celeba/sr/bicubic_x32_00274.png}} \\

\rotatebox[origin=l]{90}{\qquad\textit{DDNM}} & {\includegraphics{images/supple/celeba/sr/ddnm_x8_274.png}}& {\includegraphics{images/supple/celeba/sr/ddnm_x16_274.png}}& {\includegraphics{images/supple/celeba/sr/ddnm_x32_274.png}} \\

\rotatebox[origin=l]{90}{\qquad\textit{\methodName}} & {\includegraphics{images/supple/celeba/sr/ours_x8_274.png}}& {\includegraphics{images/supple/celeba/sr/ours_x16_274.png}}& {\includegraphics{images/supple/celeba/sr/ours_x32_274.png}} \\

 & & {\includegraphics{images/supple/celeba/sr/00274.png}}& \\
 &  & \textit{GT} &  \\

   \end{tabular}
% \caption{Visual results of super-resolution with different factors on Imagenet.}
% \caption{}
\label{fig:supres_celeba} 
}
\hfill
\setkeys{Gin}{width=0.16\linewidth}
\setlength\tabcolsep{1.pt}
\subfigure{
    \small
  \begin{tabular}{lccc}

  & \textit{$\times$4} & \textit{$\times$8} & \textit{ $\times$16 } \\
\rotatebox[origin=l]{90}{\qquad\textit{Bicubic}} & 
{\includegraphics{images/supple/imagenet/sr/bicubic_x4_1434.png}}& {\includegraphics{images/supple/imagenet/sr/bicubic_x8_1434.png}}& {\includegraphics{images/supple/imagenet/sr/bicubic_x16_1434.png}} \\

\rotatebox[origin=l]{90}{\qquad\textit{DDNM}} & 
{\includegraphics{images/supple/imagenet/sr/ddnm_1434_x4.png}}& {\includegraphics{images/supple/imagenet/sr/ddnm_1434_x8.png}}& {\includegraphics{images/supple/imagenet/sr/ddnm_1434_x16.png}} \\

\rotatebox[origin=l]{90}{\qquad\textit{\methodName}} &
{\includegraphics{images/supple/imagenet/sr/ours_1434_x4.png}}& {\includegraphics{images/supple/imagenet/sr/ours_1434_x8.png}}& {\includegraphics{images/supple/imagenet/sr/ours_1434_x16.png}} \\

 & & {\includegraphics{images/supple/imagenet/sr/1434.png}}& \\
 &  & \textit{GT} &  \\
\end{tabular}


% \caption{ Visual results of super-resolution with different factors on CelebA. Our method outputs sharper images. }
% \caption{ImageNet}
\label{fig:supres_IN}
}
\caption{Visual results of super-resolution with different upsampling factors.}
\label{fig:supres1}
\end{figure}





%%%%%%%%%% SR updated Figure %%%%%%%%%%%%%%%
\begin{figure}[t]

\setkeys{Gin}{width=0.16\linewidth}
\setlength\tabcolsep{1.pt}
    % \captionsetup[subfigure]{skip=0.5ex,
    %                          belowskip=0.5ex,
    %                          labelformat=simple}
    % \renewcommand\thesubfigure{}
    % \setlength\tabcolsep{1.pt}
    
\subfigure{
\centering
    \small
  \begin{tabular}{lccc}

  & \textit{$\times$8} & \textit{$\times$16} & \textit{ $\times$32 } \\
\rotatebox[origin=l]{90}{\qquad\textit{Bicubic}} & {\includegraphics{images/supple/celeba/sr/bicubic_x8_00282.png}}& {\includegraphics{images/supple/celeba/sr/bicubic_x16_00282.png}}& {\includegraphics{images/supple/celeba/sr/bicubic_x32_00282.png}} \\

\rotatebox[origin=l]{90}{\qquad\textit{DDNM}} & {\includegraphics{images/supple/celeba/sr/ddnm_x8_282.png}}& {\includegraphics{images/supple/celeba/sr/ddnm_x16_282.png}}& {\includegraphics{images/supple/celeba/sr/ddnm_x32_282.png}} \\

\rotatebox[origin=l]{90}{\qquad\textit{\methodName}} & {\includegraphics{images/supple/celeba/sr/ours_x8_282.png}}& {\includegraphics{images/supple/celeba/sr/ours_x16_282.png}}& {\includegraphics{images/supple/celeba/sr/ours_x32_282.png}} \\

& & {\includegraphics{images/supple/celeba/sr/00282.png}}& \\
 &  & \textit{GT} &  \\
\end{tabular}
% \caption{Visual results of super-resolution with different factors on Imagenet.}
% \caption{}
\label{fig:supres_celeb} 
}
\hfill
\setkeys{Gin}{width=0.16\linewidth}
\setlength\tabcolsep{1.pt}
\subfigure{
    \small
  \begin{tabular}{lccc}

  & \textit{$\times$4} & \textit{$\times$8} & \textit{ $\times$16 } \\
\rotatebox[origin=l]{90}{\qquad\textit{Bicubic}} & {\includegraphics{images/supple/imagenet/sr/bicubic_x4_690.png}}& {\includegraphics{images/supple/imagenet/sr/bicubic_x8_690.png}}& {\includegraphics{images/supple/imagenet/sr/bicubic_x16_690.png}} \\

\rotatebox[origin=l]{90}{\qquad\textit{DDNM}} & {\includegraphics{images/supple/imagenet/sr/ddnm_x4_690.png}}& {\includegraphics{images/supple/imagenet/sr/ddnm_x8_690.png}}& {\includegraphics{images/supple/imagenet/sr/ddnm_x16_690.png}} \\

\rotatebox[origin=l]{90}{\qquad\textit{\methodName}} & {\includegraphics{images/supple/imagenet/sr/ours_x4_690.png}}& {\includegraphics{images/supple/imagenet/sr/ours_x8_690.png}}& {\includegraphics{images/supple/imagenet/sr/ours_x16_690.png}} \\

& & {\includegraphics{images/supple/imagenet/sr/690.png}}& \\
 &  & \textit{GT} &  \\ 
\end{tabular}
% \caption{ Visual results of super-resolution with different factors on CelebA. Our method outputs sharper images. }
% \caption{ImageNet}
\label{fig:supres_IN}
}
\caption{Visual results of super-resolution with different upsampling factors.}
\label{fig:supres2}
\end{figure}



%%%%%%%%%% SR updated Figure %%%%%%%%%%%%%%%
\begin{figure}[t]

\setkeys{Gin}{width=0.16\linewidth}
\setlength\tabcolsep{1.pt}
    % \captionsetup[subfigure]{skip=0.5ex,
    %                          belowskip=0.5ex,
    %                          labelformat=simple}
    % \renewcommand\thesubfigure{}
    % \setlength\tabcolsep{1.pt}
    
\subfigure{
\centering
    \small
  \begin{tabular}{lccc}

  & \textit{$\times$8} & \textit{$\times$16} & \textit{ $\times$32 } \\
\rotatebox[origin=l]{90}{\qquad\textit{Bicubic}} & {\includegraphics{images/supple/celeba/sr/bicubic_x8_00287.png}}& {\includegraphics{images/supple/celeba/sr/bicubic_x16_00287.png}}& {\includegraphics{images/supple/celeba/sr/bicubic_x32_00287.png}} \\

\rotatebox[origin=l]{90}{\qquad\textit{DDNM}} & {\includegraphics{images/supple/celeba/sr/ddnm_x8_287.png}}& {\includegraphics{images/supple/celeba/sr/ddnm_x16_287.png}}& {\includegraphics{images/supple/celeba/sr/ddnm_x32_287.png}} \\

\rotatebox[origin=l]{90}{\qquad\textit{\methodName}} & {\includegraphics{images/supple/celeba/sr/ours_x8_287.png}}& {\includegraphics{images/supple/celeba/sr/ours_x16_287.png}}& {\includegraphics{images/supple/celeba/sr/ours_x32_287.png}} \\

& & {\includegraphics{images/supple/celeba/sr/00287.png}}& \\
 &  & \textit{GT} &  \\
   \end{tabular}
% \caption{Visual results of super-resolution with different factors on Imagenet.}
% \caption{}
\label{fig:supres_celeba} 
}
\hfill
\setkeys{Gin}{width=0.16\linewidth}
\setlength\tabcolsep{1.pt}
\subfigure{
    \small
  \begin{tabular}{lccc}

  & \textit{$\times$4} & \textit{$\times$8} & \textit{ $\times$16 } \\
\rotatebox[origin=l]{90}{\qquad\textit{Bicubic}} & {\includegraphics{images/supple/imagenet/sr/bicubic_x4_1288.png}}& {\includegraphics{images/supple/imagenet/sr/bicubic_x8_1288.png}}& {\includegraphics{images/supple/imagenet/sr/bicubic_x16_1288.png}} \\

\rotatebox[origin=l]{90}{\qquad\textit{DDNM}} & {\includegraphics{images/supple/imagenet/sr/ddnm_x4_1288.png}}& {\includegraphics{images/supple/imagenet/sr/ddnm_x8_1288.png}}& {\includegraphics{images/supple/imagenet/sr/ddnm_x16_1288.png}} \\

\rotatebox[origin=l]{90}{\qquad\textit{\methodName}} & {\includegraphics{images/supple/imagenet/sr/ours_x4_1288.png}}& {\includegraphics{images/supple/imagenet/sr/ours_x8_1288.png}}& {\includegraphics{images/supple/imagenet/sr/ours_x16_1288.png}} \\

& & {\includegraphics{images/supple/imagenet/sr/1288.png}}& \\
 &  & \textit{GT} &  \\
\end{tabular}
% \caption{ Visual results of super-resolution with different factors on CelebA. Our method outputs sharper images. }
% \caption{ImageNet}
\label{fig:supres_IN}
}
\caption{Visual results of super-resolution with different upsampling factors.}
\label{fig:supres3}
\end{figure}



\begin{figure}[h]

    \setkeys{Gin}{width=0.16\linewidth}
    \captionsetup[subfigure]{skip=0.5ex,
                             belowskip=0.5ex,
                             labelformat=simple}
    \renewcommand\thesubfigure{}
    \setlength\tabcolsep{1.pt}
    %\setlength\baselineskip{0.5pt}
    \small
    \centering
  \begin{tabular}{lcccccc}

  &\textit{Masked} & \textit{Repaint} & \textit{ DDRM } &\textit{DDNM} & \textit{\methodName} & \textit{ GT } \\
\rotatebox[origin=l]{90}{\qquad\textit{5 \%}} & 
{\includegraphics{images/supple/celeba/cs/masked_249_5_percent.png}}& {\includegraphics{images/supple/celeba/cs/repaint_249_5_percent.png}}& {\includegraphics{images/supple/celeba/cs/ddrm_249_5_percent.png}} & {\includegraphics{images/supple/celeba/cs/ddnm_249_5_percent.png}}& {\includegraphics{images/supple/celeba/cs/ours_249_5_percent.png}}& {\includegraphics{images/supple/celeba/cs/249.png}} \\
 % & \textit{18.72} & \textit{31.30} & \textit{31.38} & \textit{31.25} & \textbf{\textit{31.46}} \\
%\vspace{-1cm}
\rotatebox[origin=l]{90}{\qquad\textit{1 \%}} & 
{\includegraphics{images/supple/celeba/cs/masked_249_1_percent.png}}& {\includegraphics{images/supple/celeba/cs/repaint_249_1_percent.png}}& {\includegraphics{images/supple/celeba/cs/ddrm_249_1_percent.png}} & {\includegraphics{images/supple/celeba/cs/ddnm_249_1_percent.png}}& {\includegraphics{images/supple/celeba/cs/ours_249_1_percent.png}}& {\includegraphics{images/supple/celeba/cs/249.png}} \\

\rotatebox[origin=l]{90}{\qquad\textit{5 \%}} & 
{\includegraphics{images/supple/celeba/cs/masked_285_5_percent.png}}& {\includegraphics{images/supple/celeba/cs/repaint_285_5_percent.png}}& {\includegraphics{images/supple/celeba/cs/ddrm_285_5_percent.png}} & {\includegraphics{images/supple/celeba/cs/ddnm_285_5_percent.png}}& {\includegraphics{images/supple/celeba/cs/ours_285_5_percent.png}}& {\includegraphics{images/supple/celeba/cs/285.png}} \\


\rotatebox[origin=l]{90}{\qquad\textit{1 \%}} & 
{\includegraphics{images/supple/celeba/cs/masked_285_1_percent.png}}& {\includegraphics{images/supple/celeba/cs/repaint_285_1_percent.png}}& {\includegraphics{images/supple/celeba/cs/ddrm_285_1_percent.png}} & {\includegraphics{images/supple/celeba/cs/ddnm_285_1_percent.png}}& {\includegraphics{images/supple/celeba/cs/ours_285_1_percent.png}}& {\includegraphics{images/supple/celeba/cs/285.png}} \\

\rotatebox[origin=l]{90}{\qquad\textit{5 \%}} & 
{\includegraphics{images/supple/celeba/cs/masked_458_5_percent.png}}& {\includegraphics{images/supple/celeba/cs/repaint_458_5_percent.png}}& {\includegraphics{images/supple/celeba/cs/ddrm_458_5_percent.png}} & {\includegraphics{images/supple/celeba/cs/ddnm_458_5_percent.png}}& {\includegraphics{images/supple/celeba/cs/ours_458_5_percent.png}}& {\includegraphics{images/supple/celeba/cs/00458.png}} \\

\rotatebox[origin=l]{90}{\qquad\textit{1 \%}} & 
{\includegraphics{images/supple/celeba/cs/masked_458_1_percent.png}}& {\includegraphics{images/supple/celeba/cs/repaint_458_1_percent.png}}& {\includegraphics{images/supple/celeba/cs/ddrm_458_1_percent.png}} & {\includegraphics{images/supple/celeba/cs/ddnm_458_1_percent.png}}& {\includegraphics{images/supple/celeba/cs/ours_458_1_percent.png}}& {\includegraphics{images/supple/celeba/cs/00458.png}} \\

   \end{tabular}
% \captionof{figure}{\label{fig:inpainting} Visual results of inpaintings }
\caption{Visual results of CS on CelebA.}
\label{fig:cs1} 
\end{figure}



\begin{figure}[h]

    \setkeys{Gin}{width=0.16\linewidth}
    \captionsetup[subfigure]{skip=0.5ex,
                             belowskip=0.5ex,
                             labelformat=simple}
    \renewcommand\thesubfigure{}
    \setlength\tabcolsep{1.pt}
    %\setlength\baselineskip{0.5pt}
    \small
    \centering
  \begin{tabular}{lcccccc}

  &\textit{Masked} & \textit{Repaint} & \textit{ DDRM } &\textit{DDNM} & \textit{\methodName} & \textit{ GT } \\
\rotatebox[origin=l]{90}{\qquad\textit{5 \%}} & 
{\includegraphics{images/supple/imagenet/cs/masked_94_5_percent.png}}& {\includegraphics{images/supple/imagenet/cs/repaint_94_5_percent.png}}& {\includegraphics{images/supple/imagenet/cs/ddrm_94_5_percent.png}} & {\includegraphics{images/supple/imagenet/cs/ddnm_94_5_percent.png}}& {\includegraphics{images/supple/imagenet/cs/ours_94_5_percent.png}}& {\includegraphics{images/supple/imagenet/cs/94.png}} \\
 % & \textit{18.72} & \textit{31.30} & \textit{31.38} & \textit{31.25} & \textbf{\textit{31.46}} \\
%\vspace{-1cm}
\rotatebox[origin=l]{90}{\qquad\textit{1 \%}} & 
{\includegraphics{images/supple/imagenet/cs/masked_94_1_percent.png}}& {\includegraphics{images/supple/imagenet/cs/repaint_94_1_percent.png}}& {\includegraphics{images/supple/imagenet/cs/ddrm_94_1_percent.png}} & {\includegraphics{images/supple/imagenet/cs/ddnm_94_1_percent.png}}& {\includegraphics{images/supple/imagenet/cs/ours_94_1_percent.png}}& {\includegraphics{images/supple/imagenet/cs/94.png}} \\

\rotatebox[origin=l]{90}{\qquad\textit{5 \%}} & 
{\includegraphics{images/supple/imagenet/cs/masked_247_5_percent.png}}& {\includegraphics{images/supple/imagenet/cs/repaint_247_5_percent.png}}& {\includegraphics{images/supple/imagenet/cs/ddrm_247_5_percent.png}} & {\includegraphics{images/supple/imagenet/cs/ddnm_247_5_percent.png}}& {\includegraphics{images/supple/imagenet/cs/ours_247_5_percent.png}}& {\includegraphics{images/supple/imagenet/cs/247.png}} \\


\rotatebox[origin=l]{90}{\qquad\textit{1 \%}} & 
{\includegraphics{images/supple/imagenet/cs/masked_247_1_percent.png}}& {\includegraphics{images/supple/imagenet/cs/repaint_247_1_percent.png}}& {\includegraphics{images/supple/imagenet/cs/ddrm_247_1_percent.png}} & {\includegraphics{images/supple/imagenet/cs/ddnm_247_1_percent.png}}& {\includegraphics{images/supple/imagenet/cs/ours_247_1_percent.png}}& {\includegraphics{images/supple/imagenet/cs/247.png}} \\

\rotatebox[origin=l]{90}{\qquad\textit{5 \%}} & 
{\includegraphics{images/supple/imagenet/cs/masked_975_5_percent.png}}& {\includegraphics{images/supple/imagenet/cs/repaint_975_5_percent.png}}& {\includegraphics{images/supple/imagenet/cs/ddrm_975_5_percent.png}} & {\includegraphics{images/supple/imagenet/cs/ddnm_975_5_percent.png}}& {\includegraphics{images/supple/imagenet/cs/ours_975_5_percent.png}}& {\includegraphics{images/supple/imagenet/cs/975.png}} \\

\rotatebox[origin=l]{90}{\qquad\textit{1 \%}} & 
{\includegraphics{images/supple/imagenet/cs/masked_975_1_percent.png}}& {\includegraphics{images/supple/imagenet/cs/repaint_975_1_percent.png}}& {\includegraphics{images/supple/imagenet/cs/ddrm_975_1_percent.png}} & {\includegraphics{images/supple/imagenet/cs/ddnm_975_1_percent.png}}& {\includegraphics{images/supple/imagenet/cs/ours_975_1_percent.png}}& {\includegraphics{images/supple/imagenet/cs/975.png}} \\

   \end{tabular}
% \captionof{figure}{\label{fig:inpainting} Visual results of inpaintings }
\caption{Visual results of CS on ImageNet.}
\label{fig:cs2} 
\end{figure}


\begin{figure}[h]
    \setkeys{Gin}{width=0.16\linewidth}
    \captionsetup[subfigure]{skip=0.5ex,
                             belowskip=0.5ex,
                             labelformat=simple}
    \renewcommand\thesubfigure{}
    \setlength\tabcolsep{1.pt}
    %\setlength\baselineskip{0.5pt}
    \small
    \centering
  \begin{tabular}{cccccc}

   \textit{Blurry} & \textit{SelfDeblur} & \textit{OID}& \textit{Chen et al.} & \textit{ \methodName }& \textit{ GT } \\

   %\rotatebox[origin=l]{90}{\qquad\textit{ImageNet}} & 
{\includegraphics{images/supple/celeba/deblur/blurry_341.png}}& {\includegraphics{images/supple/celeba/deblur/selfdeblur_341.png}}&
{\includegraphics{images/supple/celeba/deblur/oid_321.png}}& 
{\includegraphics{images/supple/celeba/deblur/341_celeba.png}}& 
{\includegraphics{images/supple/celeba/deblur/ours_341.png}}& {\includegraphics{images/supple/celeba/deblur/gt_341.png}} \\
%\rotatebox[origin=l]{90}{\qquad\textit{ CelebA}} & 
{\includegraphics{images/supple/celeba/deblur/blurry_328.png}}& {\includegraphics{images/supple/celeba/deblur/self2self_328.png}}& 
{\includegraphics{images/supple/celeba/deblur/oid_328.png}}& 
{\includegraphics{images/supple/celeba/deblur/328_celeba.png}}& 
{\includegraphics{images/supple/celeba/deblur/ours_328.png}}& {\includegraphics{images/supple/celeba/deblur/gt_328.png}} \\

{\includegraphics{images/supple/celeba/deblur/blurry_377.png}}& {\includegraphics{images/supple/celeba/deblur/selfdeblur_377.png}}& 
{\includegraphics{images/supple/celeba/deblur/oid_377.png}}& 
{\includegraphics{images/supple/celeba/deblur/377_celeba.png}}& 
{\includegraphics{images/supple/celeba/deblur/ours_377.png}}& {\includegraphics{images/supple/celeba/deblur/gt_377.png}} \\

   \end{tabular}
\captionof{figure}{\label{fig:deblur1} Visual results of blind deconvolution using a random Gaussian kernel with size $41\times 41$ on CelebA.}
\end{figure}


\begin{figure}[h]
    \setkeys{Gin}{width=0.16\linewidth}
    \captionsetup[subfigure]{skip=0.5ex,
                             belowskip=0.5ex,
                             labelformat=simple}
    \renewcommand\thesubfigure{}
    \setlength\tabcolsep{1.pt}
    %\setlength\baselineskip{0.5pt}
    \small
    \centering
  \begin{tabular}{cccccc}

   \textit{Blurry} & \textit{SelfDeblur} & \textit{OID} & \textit{Chen et al.} &\textit{ \methodName }& \textit{ GT } \\

   %\rotatebox[origin=l]{90}{\qquad\textit{ImageNet}} & 
{\includegraphics{images/supple/imagenet/deblur/blurry_img1.png}}& {\includegraphics{images/supple/imagenet/deblur/selfdeblur_291.png}}& 
{\includegraphics{images/supple/imagenet/deblur/oid_img1.png}}& 
{\includegraphics{images/supple/imagenet/deblur/img1_imagenet.png}}& 
{\includegraphics{images/supple/imagenet/deblur/ours_291.png}}& {\includegraphics{images/supple/imagenet/deblur/gt_291.png}} \\
%\rotatebox[origin=l]{90}{\qquad\textit{ CelebA}} & 

{\includegraphics{images/supple/imagenet/deblur/blurry_img2.png}}& {\includegraphics{images/supple/imagenet/deblur/selfdeblur_423.png}}& 
{\includegraphics{images/supple/imagenet/deblur/oid_img2.png}}& 
{\includegraphics{images/supple/imagenet/deblur/img2_imagenet.png}}& 
{\includegraphics{images/supple/imagenet/deblur/ours_423.png}}& {\includegraphics{images/supple/imagenet/deblur/gt_423.png}} \\

{\includegraphics{images/supple/imagenet/deblur/blurry_img3.png}}& {\includegraphics{images/supple/imagenet/deblur/selfdeblur_1067.png}}&
{\includegraphics{images/supple/imagenet/deblur/oid_img3.png}}& 
{\includegraphics{images/supple/imagenet/deblur/img3_imagenet.png}}& 
{\includegraphics{images/supple/imagenet/deblur/ours_1067.png}}& {\includegraphics{images/supple/imagenet/deblur/gt_1067.png}} \\

   \end{tabular}
\captionof{figure}{\label{fig:deblur2} Visual results of blind deconvolution using a random Gaussian kernel with size $41\times 41$ on ImageNet.}
\end{figure}

\FloatBarrier


{\small
\bibliographystyle{plain}
\bibliography{egbib}
}

%%%%%%%%%%%%%%%%%%%%%%%%%%%%%%%%%%%%%%%%%%%%%%%%%%%%%%%%%%%%
\textbf{Q1. Core approach discussed in Section 3.2.3, eq(19), eq(21), eq(22)}

Here we provide a more theoretical analysis of the approach discussed in Section 3.2.3 and comment on eq(19), eq(21), and eq(22).

First, we want to note that the derivation in Section 3.2.3 is directly connected to our problem formulation in eq (8). Indeed, what we do is simply solving eq (8). Here is eq(8):

$$
\hat{x} = \arg\min_{z: \|z\|^2 = N_x M_x} \| y - H(g(z)) \|^2
$$

One challenge in solving eq(8) is that an iterative approach can be computationally expensive, as a single evaluation of $g(z)$ may take minutes.

In this context, eq(19) introduces a family of generative processes $\text{DDIMReverse}(., \delta t) = g^{\delta t}$ parameterized by $\delta t \geq 1$. These are defined not on all latent variables $x_{1:T}$, but on a subset $\{x_0, x_{\delta t}, x_{2 \delta t}, \ldots, x_{T-2 \delta t}, x_{T-\delta t}, x_T\}$ of length $K$. $\delta t$ is a scalar that defines a jump in the generative process sampling.

By carefully factorizing both the diffusion forward process and the generative process, and defining the marginals, we can show that $g^{\delta t \geq 1}$ constitutes a valid generative model for $p(x)$.

Here is a brief derivation:

\vspace{0.3 cm}

We consider the following factorization of the diffusion forward process:

$$
q_{\delta t}(x_{1:T} | x_0) = \prod_{i=1}^{K} q_{\delta t}(x_{(i -1) \delta t} | x_{i \delta t}, x_0) \prod_{t \notin \tau} q_{\delta t}(x_t | x_0)
$$

where

$$
q_{\delta t}(x_t | x_0) = \mathcal{N} \left( \sqrt{\bar{\alpha_t}} x_0, (1 - \bar{\alpha_t}) I \right)
$$

and

$$
q_{\delta t}(x_{(i -1) \delta t} | x_{i \delta t}, x_0) = \mathcal{N} \left( \sqrt{\bar{\alpha_{t-1}}} x_0 + \sqrt{1 - \bar{\alpha_{t-1}} - \sigma_t^2} \frac{x_t - \sqrt{\bar{\alpha_t}} x_0}{\sqrt{1 - \bar{\alpha_t}}}, \sigma_t^2 I \right)
$$

Particularly, $q_{\delta t}(x_{t-1} | x_t, x_0)$ is defined such that $q_{\delta t}(x_{i \delta t} | x_0) = \mathcal{N} \left( \sqrt{\bar{\alpha_{i \delta t}}} x_0, (1 - \bar{\alpha_{i \delta t}}) I \right)$ for all $i \in [1, K]$. (Here, all the marginals $q_{\delta t}(x_t | x_0)$ for $t \in [1, T]$ match those in the original diffusion paper.)

We then define the corresponding generative process $p_{\theta, \delta t}$:

$$
p_{\theta, \delta t}(x_{1:T} | x_0) = \prod_{i=1}^{K} p_{\theta, \delta t}(x_{(i -1) \delta t} | x_{i \delta t}) \prod_{t \notin \tau} q_{\delta t}(x_t | x_0)
$$

(where only the first part of the factorization will be used to produce samples).

We define

$$
p_{\theta, \delta t}(x_0 | x_t) = \mathcal{N} \left( f_{\theta}^{(t)}(x_t), \sigma_t^2 I \right)
$$

and

$$
p_{\theta, \delta t}(x_{(i -1) \delta t} | x_{i \delta t}) = q_{\delta t}(x_{(i -1) \delta t} | x_{i \delta t}, f_{\theta}^{(i \delta t)}(x_{(i -1) \delta t}))
$$

where

$$
f_{\theta}^{(t)}(x_t) = \frac{x_t - \sqrt{1 - \alpha_t} \cdot \epsilon_\theta^{(t)}(x_t)}{\sqrt{\alpha_t}}
$$

We optimize $\theta$ using the following variational inference objective:

$$
J(\epsilon_\theta) = \mathbb{E_{x_{0:T} \sim q_{\delta t} (x_{0:T})}} \left[ \log q_{\delta t} (x_{1:T} | x_0) - \log p_{\theta, \delta t} (x_{0:T}) \right]
$$

$$
= \mathbb{E_{x_{0:T} \sim q_{\delta t} (x_{0:T})}} \left[ \sum_{i=1}^{K} D_{KL} \left(q_{\delta t} (x_{(i -1) \delta t} | x_{i \delta t}, x_0) \, \| \, p_{\theta, \delta t} (x_{(i -1) \delta t} | x_{i \delta t}) \right) + \sum_{t \notin \tau} D_{KL} \left(q_{\delta t} (x_t | x_0) \, \| \, p_{\theta, \delta t} (x_0 | x_t) \right) \right]
$$

where each KL divergence is between two Gaussians where only the mean depends on $\theta$.

By substituting all the terms with their values:

$$
J(\epsilon_\theta) = \mathbb{E_{t \sim \mathcal{U}(0, 1); x_0 \sim q(x); \epsilon \sim \mathcal{N}(0, I)}} \left[ \| \epsilon - \epsilon_{\theta} (\sqrt{\bar{\alpha_t}} x_0 + \sqrt{1 - \bar{\alpha_t}} \epsilon, t) \|^2 \right]
$$

This is the original training objective of the diffusion model (defined on all the time-steps $[1, T]$). This means that:

1) All the generative processes $g^{\delta t}$ are equivalent and can be used to sample from $p(x)$.
2) There is no need to retrain, as the training objective for the generative process involving only a subset is the same for all processes.

Based on these results, we can rewrite the minimization in eq(8) as:

$$
\hat{x} = \arg\min_{z: \|z\|^2 = N_x M_x} \| y - H(g^{\delta t \gg 1}(z)) \|^2
$$

This will lead to a much more efficient evaluation of the objective while remaining equivalent to eq(8).


\end{document}
